# Supplementary material for: Terahertz Time-Domain Spectroscopy and Density Functional Theory Analysis of Low-Frequency Vibrational Modes of a Benzoxazolium-Coumarin Donor-pi-Acceptor Chromophore
Source: arXiv:2510.25365 ancillary file (2025-12-14)
Supplement: Supplementary file 1 [file SupportingInformation.pdf]

**Supporting Information:**

**Terahertz Time-Domain Spectroscopy and  
Density Functional Theory Analysis of  
Low-Frequency Vibrational Modes of a  
Benzoxazolium–Coumarin Donor– $\pi$ –Acceptor  
Chromophore**

Sidhanta Sahu,<sup>†,§</sup> Phalguna Krishna Das Vana,<sup>†,§</sup> Anupama Chauhan,<sup>†</sup> Poulami  
Ghosh,<sup>†</sup> Vijay Sai Krishna Cheerla,<sup>‡</sup> Sanyam,<sup>¶</sup> C. N. Sundaresan,<sup>‡</sup> and N.  
Kamaraju<sup>\*,†</sup>

<sup>†</sup>*Department of Physical Sciences, Indian Institute of Science Education and Research  
Kolkata, Mohanpur, West Bengal 741246, India.*

<sup>‡</sup>*Department of Chemistry, Sri Sathya Sai Institute of Higher Learning, Brindavan  
Campus, Kadugodi, Bangalore 560067, India.*

<sup>¶</sup>*Department of Chemistry, Indian Institute of Technology Gandhinagar, Gandhinagar,  
Gujarat 382355, India.*

<sup>§</sup>*These authors contributed equally to this work.*

E-mail: nkamaraju@iiserkol.ac.in

# Contents

|                                                     |            |
|-----------------------------------------------------|------------|
| <b>S1 Characterization</b>                          | <b>S-3</b> |
| S1.1 NMR . . . . .                                  | S-3        |
| S1.2 Additional Steady-State Spectroscopy . . . . . | S-4        |
| <b>S2 THz–TDS</b>                                   | <b>S-5</b> |
| S2.1 Thickness Measurements . . . . .               | S-5        |
| S2.2 Repeatability . . . . .                        | S-5        |
| <b>S3 Global Frequency Scaling</b>                  | <b>S-6</b> |
| <b>S4 Movies of simulated vibrational modes</b>     | <b>S-7</b> |

# S1 Characterization

## S1.1 NMR

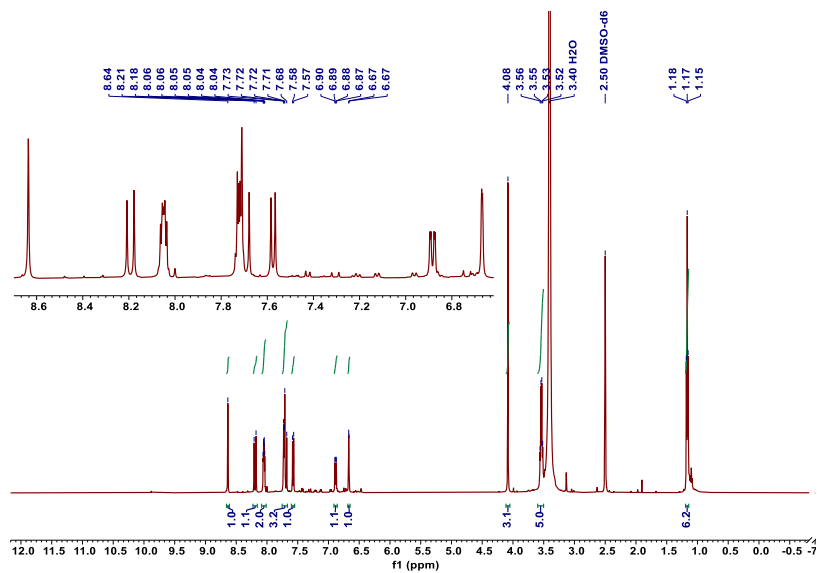

Figure S1: <sup>1</sup>H NMR spectrum with key assignments.

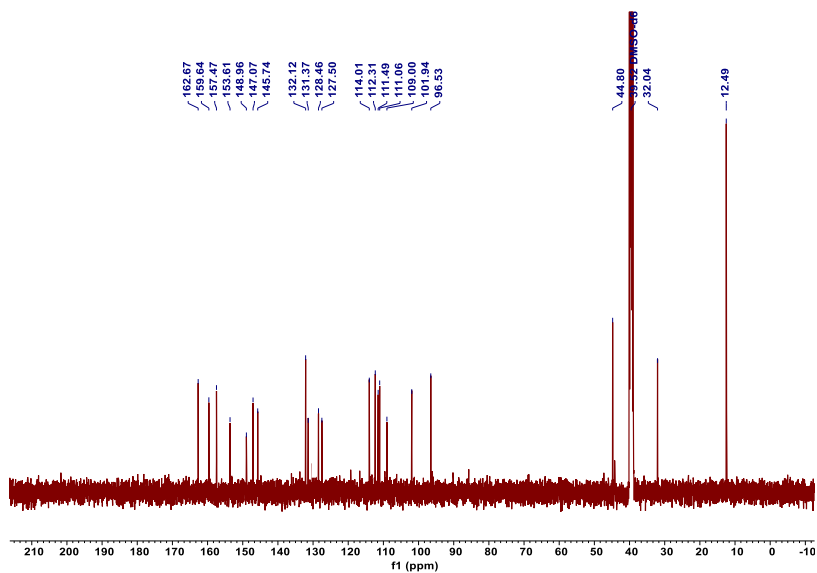

Figure S2: <sup>13</sup>C NMR spectrum with key assignments.

## S1.2 Additional Steady-State Spectroscopy

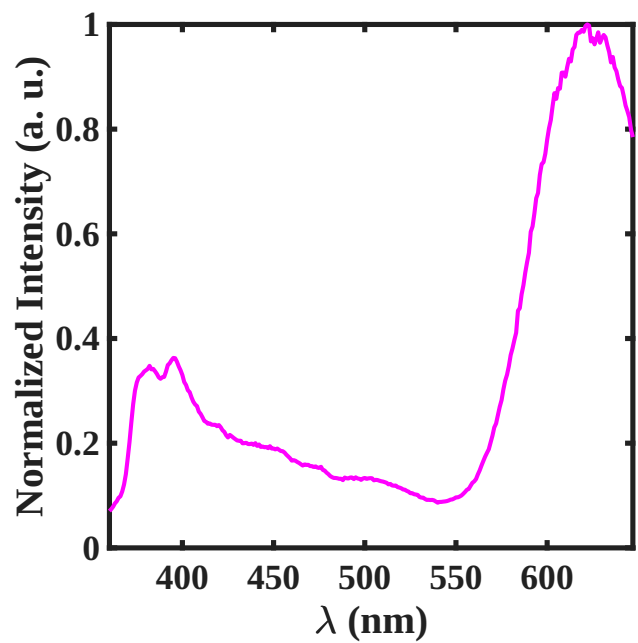

Figure S3: Emission spectrum (excitation at 340 nm).

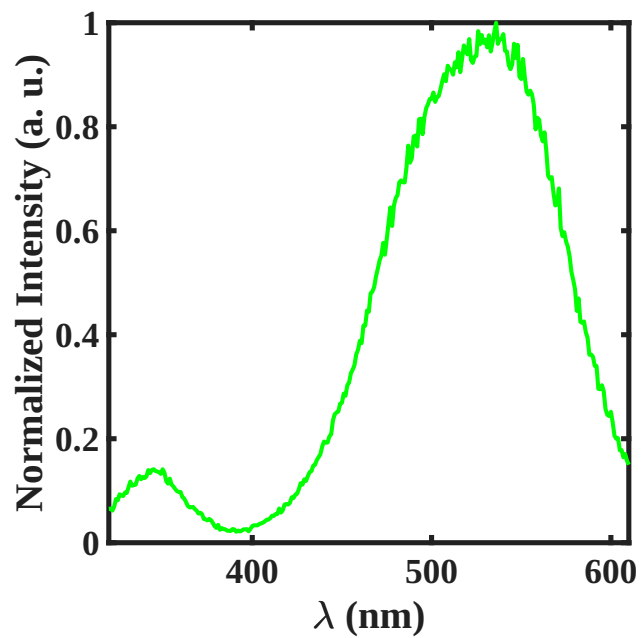

Figure S4: Emission intensity at 620 nm versus excitation wavelength.

## S2 THz–TDS

### S2.1 Thickness Measurements

Thickness was measured at multiple positions on the pellet with a micrometer (resolution 1  $\mu\text{m}$ ). Units are  $\mu\text{m}$ . The raw values and descriptive statistics are summarized below.

Table S1: Pellet thickness values.

| Pos. 1 | Pos. 2 | Pos. 3 | Pos. 4 | Pos. 5 | Pos. 6 |
|--------|--------|--------|--------|--------|--------|
| 454.0  | 463.0  | 464.0  | 463.0  | 447.0  | 462.0  |

**Summary:** Mean = 458.8  $\mu\text{m}$ ; SD = 6.9  $\mu\text{m}$ ; 95% CI half-width = 5.48  $\mu\text{m}$ ; Range = 447.0–464.0  $\mu\text{m}$ ;  $N = 6$ .

### S2.2 Repeatability

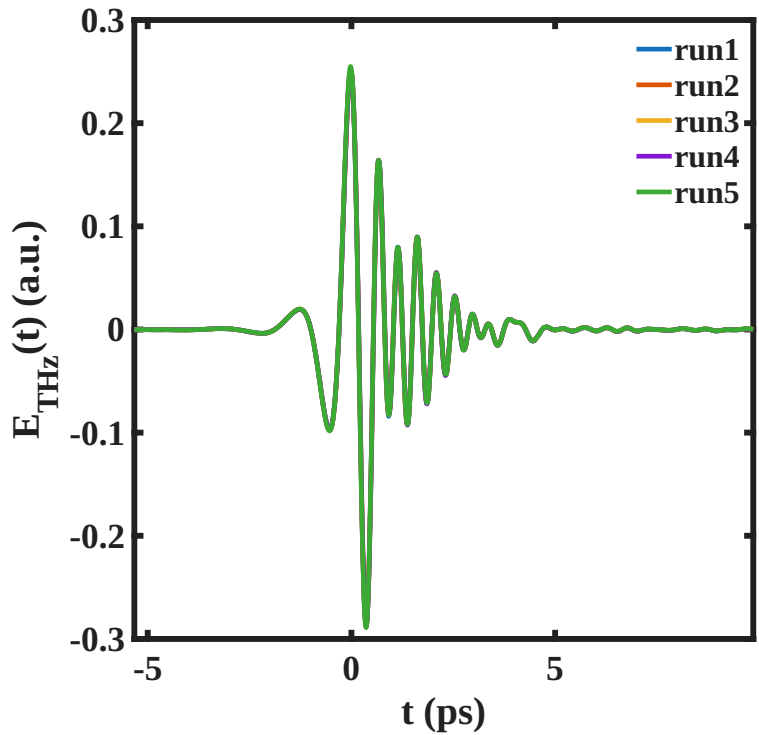

Figure S5: Repeatability of the time-domain THz waveform for the air reference. Five independent runs (run1–run5) are overlaid.

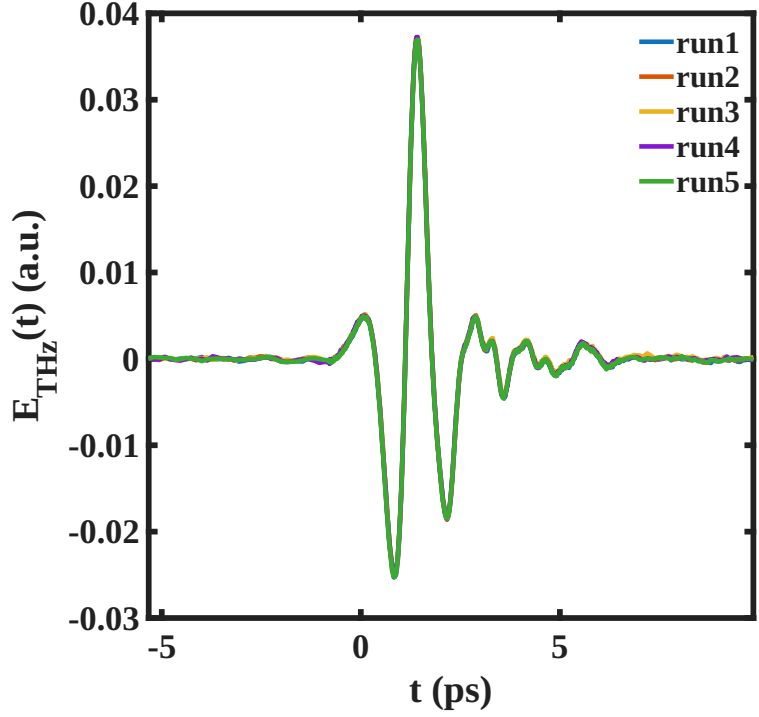

Figure S6: Repeatability of the time-domain THz waveform for the  $\text{BCO}^+$  sample. Five independent runs (run1–run5) are overlaid.

### S3 Global Frequency Scaling

Single anchor:  $s_{\text{anchor}} = 1.300/1.047 = 1.2416$ . Least-squares across five peaks:  $s^* = 1.24$ , RMSE = 0.0145 THz.

Table S2: Matched peaks used for scaling.

| Peak ID                          | $\nu_{\text{obs}}$ (THz) | $\nu_{\text{calc}}$ (THz) |
|----------------------------------|--------------------------|---------------------------|
| P_E1 / P_S1                      | 0.62                     | 0.52                      |
| P_E2 / P_S2                      | 0.85                     | 0.68                      |
| P_E3 / P_S3                      | 1.30                     | 1.04                      |
| P_E4 / P_S4                      | 1.81                     | 1.45                      |
| P_E5 / P_S5                      | 2.07                     | 1.68                      |
| $s^* = 1.24$ , RMSE = 0.0145 THz |                          |                           |

# S4 Movies of simulated vibrational modes

Gas-phase DFT normal modes typically overestimate solid-state frequencies; we therefore apply a single global frequency scale factor  $s$  to the calculated modes. We determine  $s$  by (i) an anchor-based ratio using a high-SNR, unambiguous peak pair and (ii) a least-squares fit over five matched peaks minimizing RMSE in THz. Both approaches yield nearly the same value (Table S2). Mode visualizations with top- and side-view animations are provided as SI Movies S1–S6.

Table S3: Peaks  $P_{S1}$ – $P_{S5}$  and SI movie files.

| Peaks              | SI movie files                                     |
|--------------------|----------------------------------------------------|
| $P_{S1}$           | S1_top.gif / S1_side.gif                           |
| $P_{S2}$           | S2_top.gif / S2_side.gif                           |
| $P_{S3}$ (doublet) | S3_top.gif / S3_side.gif; S4_top.gif / S4_side.gif |
| $P_{S4}$           | S5_top.gif / S5_side.gif                           |
| $P_{S5}$           | S6_top.gif / S6_side.gif                           |
